# Supplementary material for: Near-optimal Algorithms for Stochastic Online Bin Packing
Source: arXiv:2205.03622 source file (2025-03-04)
Supplement: Supplementary file 1 [file appendixIID.tex]

\section{Omitted Proofs from Section \ref{sec:iid-model}}
\label{app:iid}
\subsection{Omitted Proof of \cref{rhee-talagrand}}

\subsection{Omitted Proof of \cref{weight-conc}}

\subsection{Omitted Proof of \cref{large-item-conc}}

\subsection{Omitted Proof of \cref{lem:decomposition}}

%\noindent\textbf{Analysis of $\ALG(I)$ in the low probability event in Case 2 and the final competitive ratio.}
% \subsection{Exact Competitive Ratio of \texorpdfstring{$\ALG$}{Alg}}
% \label{sec:exact-comp-ratio}
