# Supplementary material for: Near-optimal Algorithms for Stochastic Online Bin Packing
Source: arXiv:2205.03622 source file (2025-03-04)
Supplement: Supplementary file 2 [file appendixROA.tex]

\section{Details of section \ref{sec:roa}}
\label{app:3-partition}
